# Supplementary material for: Continuous-Domain Solutions of Linear Inverse Problems with Tikhonov vs. Generalized TV Regularization
Source: arXiv:1802.01344 source file (2018-02-05)
Supplement: Supplementary file 1 [file AppendixJournalMain.tex]

\subsection{Proof of Theorem \ref{theo:L2_representer}}
Since both $E$ and $\| \Lop f\|^2_{L_2} $ are convex, their sum criterion is convex as well. Therefore, (\ref{empirical}) admits a minimizer. Let $f^*$ be a minimizer. Then, it is also a solution of the problem
\begin{align*}
f^*= \arg \min \| \Lop f\|^2_{2} \\
\text{such that }\V \nu(f)\in \V \nu(f^*).
\end{align*}
The solution of this case has been discussed in \cite{bezhaev2001variational} and admits the specified representation.
Alternatively, we also prove the same here.
\begin{IEEEproof}

%\begin{align*}
%f^*= \arg \min \| \Lop f\|^2_{L_2} \\
%\text{such that } E(\V z, \V \nu(f))\leq \alpha
%\end{align*}
Let $f_{\as}$ be the projection of $f$ on the dual of the span formed by the linear measurement vectors. It then can be written as,
$$f=f_{\as}+f_{\ap}$$
both of which can be projected on $\Spc H_{\Lop, \V \phi}=\bl/\nl$ and $\nl$ as,
\begin{align*}
f_{\as}&=f_{\ah}+f_{\anl}\\
f_{\ap}&=f_{\aph}+f_{\apnl}
\end{align*}     
As $E$ and $ \| \Lop f\|^2_{L_2} $ are both convex, the resulting summation is also convex ensuring the existence of minimizer of \ref{empirical}.% Let $f^*$ be a minimizer and $E(\V z, \V \nu(f^*))=\alpha$ then, 

Let $f^*$ be the minimizer then, it can be argued that it is also a solution of,
$$f^*=\arg \min \| \Lop f\| \quad s.t. \quad \nu(f)=\nu(f^*)$$
we now show that as $f^*$ is the solution of later formulation it admits the representation specified.
Let $\nu(f^*)=z_0$, then,
\begin{align*}
\V \nu^{-1}(z_0) &= f_{\as}^{z_0}+\na\\
%\Op A^{-1}(z_0) & f_{\as}^{z_0}+{\na}_{\Spc H}+{\na}_{\nl}\\
\V \nu^{-1}(z_0) &= f_{\ah}^{z_0}+f_{\anl}^{z_0}+{\na}_{\Spc H}+{\na}_{\nl}\\
\Lop \V \nu^{-1}(z_0) &= \Lop f_{\ah}^{z_0}+\Lop {\na}_{\Spc H}\\
\end{align*}

 $\Lop {\na}_{\Spc H}$ is convex and closed and therefore, $\Lop \V \nu^{-1}(z_0)$ too and by Hilbert's projection theorem $\Lop f^* =w_0$ is the projection of $\V 0$ on the above set.
We decompose $f^*=f^*_{\Spc H_{\Lop,\V \phi}}+f^*_{\nl}$ which can be further decomposed into, $f^*=f^*_{\ah}+f^*_{\aph}+f^*_{\nl}$. Interestingly, $f^{**}=f^{*}_{\ah}+f^*_{\nl}$ is also in $\V \nu^{-1}(z_0)$, and as $f^*$ is the projection of $\V 0$ on this set therefore,
$$\|\Lop f^* \|^2 \leq \|\Lop f^{**} \|^2  $$
which implies that $f^*_{\aph}=0$. Thus, the solution is 
$$f^*=f^*_{\ah}+f^*_{\nl}$$
which admits the following representation,
\begin{equation*}\label{spline}
  f^*(\bx)=\sum_{i=1}^{M} a_i \{\Lop^{-1}_{\boldsymbol {\phi}}\{\Lop^{-1*}_{\boldsymbol {\phi}}\nu_i\}\}(\bx)+\sum_{j=1}^{N_0} b_j p_j(\bx).
  \end{equation*}
  as $\Spc {AH}$ is spanned by the projection of the dual of the measurements on the quotient space i.e. $\{\Lop^{-1}_{\boldsymbol {\phi}}\{\Lop^{-1*}_{\boldsymbol {\phi}}\nu_i\}\}_{i=1}^M$.  It then can be further argued that $$\sum_{i=1}^{M} a_i \{\Lop^{-1}_{\boldsymbol {\phi}}\{\Lop^{-1*}_{\boldsymbol {\phi}}\nu_i\}\}(\bx)= \sum_{i=1}^{M} a_i (\Lop*\Lop)^{-1}\nu_i(\bx)+p_0$$
  for some $p_0 \in \nl.$ On substituting this we get the result,
  \begin{equation*}\label{spline}
  f^*(\bx)=\sum_{i=1}^{M} a_i (\Lop*\Lop)^{-1}\nu_i(\bx)+\sum_{j=1}^{N_0} b_j p_j(\bx).
  \end{equation*}

\end{IEEEproof}

\subsection{Proof of Theorem \ref{theo:L1_representer}}
The global criterion is convex. Therefore, (\ref{empiricalL1}) admits a minimizer denoted by $f^*$. Then, it is also a solution of the problem
\begin{align*}
f^*= \arg \min \| \Lop f\|_{TV} \\
\text{such that }\V \nu(f)=\Spc C_0,
\end{align*}
where the set $\Spc C_0=\{z \in \Rm: z=\V \nu(f^*)\}$ reduces to a single point. Since $\Spc C_0$ is trivially closed, convex, and bounded, the solution of the problem admits the specified representation (by Theorem \ref{theo:L1_representerConvex}).
